# Supplementary material for: Enhanced single photon emission from carbon nanotube dopant states coupled to silicon microcavities
Source: arXiv:1803.08628 ancillary file (2018-03-23)
Supplement: Supplementary file 1 [file Supporting_Information.pdf]

# SUPPORTING INFORMATION

## Enhanced single photon emission from carbon nanotube dopant states coupled to silicon microcavities

A. Ishii[1,2], X. He[3], N. F. Hartmann[3], H. Machiya[1,4], H. Htoon[3], S. K. Doorn[3], and Y. K. Kato[1,3]

*1 Nanoscale Quantum Photonics Laboratory, RIKEN, Saitama 351-0198, Japan*
*2 Quantum Optoelectronics Research Team, RIKEN Center for Advanced Photonics, Saitama 351-0198, Japan*
*3 Center for Integrated Nanotechnologies, Materials Physics and Applications Division, Los Alamos National Laboratory, Los Alamos, New Mexico 87545, United States*
*4 Department of Electrical Engineering, The University of Tokyo, Tokyo 113-8656, Japan*

## S1. Comparison of photon antibunching with and without spectral filtering

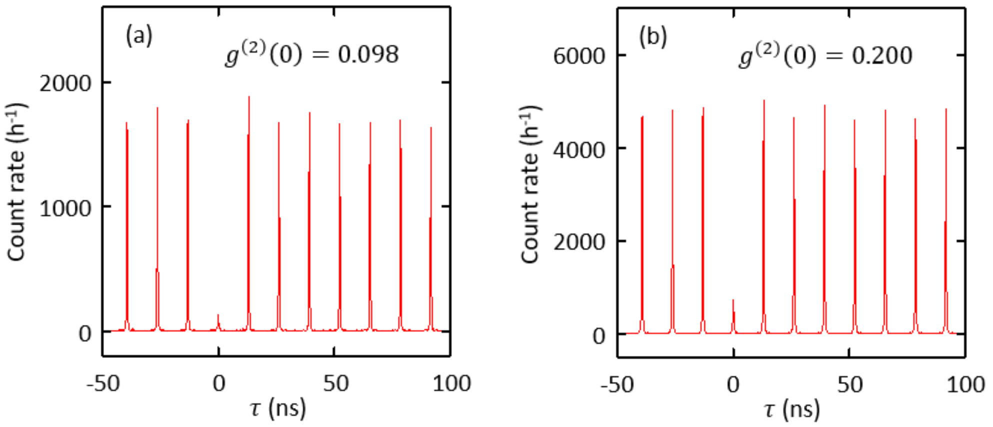


FIG. S1 Autocorrelation histograms (a) with the band-pass filter and (b) with the long-pass filter. *X*-polarized pulsed laser with $P = 0.1$ μW is used for excitation. The measurements are done on the device shown in Figs. 3(a) and (d).

## S2. Derivation of photon detection rate $\Gamma$

In the photon correlation measurements, autocorrelation counts are accumulated only when the two channels of SSPD detect photons within the same time window. Here we assume that photon detection events within a time window is one at most for each channel, where the condition is expressed as

$$\Gamma_{Ch1}, \Gamma_{Ch2} \ll \frac{1}{T}$$

where $\Gamma_{Ch1}$ and $\Gamma_{Ch2}$ are photon detection rates at channel 1 and 2, respectively, and $T$ is the time window size. Under this assumption, the autocorrelation count rate $C$ is given by

$$C = \Gamma_{Ch1} \cdot \Gamma_{Ch2} \cdot T$$

Using the signal splitting ratio $r = \Gamma_{Ch2}/\Gamma_{Ch1}$ of the optical fiber, we can express the detection rates as $\Gamma_{Ch1} = \sqrt{C/rT}$ and $\Gamma_{Ch2} = \sqrt{rC/T}$. As the total photon detection rate $\Gamma$ is the sum of $\Gamma_{Ch1}$ and $\Gamma_{Ch2}$, we obtain

$$\Gamma = \Gamma_{Ch1} + \Gamma_{Ch2} = \left(\sqrt{r} + \frac{1}{\sqrt{r}}\right)\sqrt{\frac{C}{T}}$$

We note that this relation is valid for $\Gamma < 5.65 \times 10^6$ counts/s, and our measurement results in this paper are at least one order of magnitude lower than this limit.

## S3. Observation of photon bunching at high powers

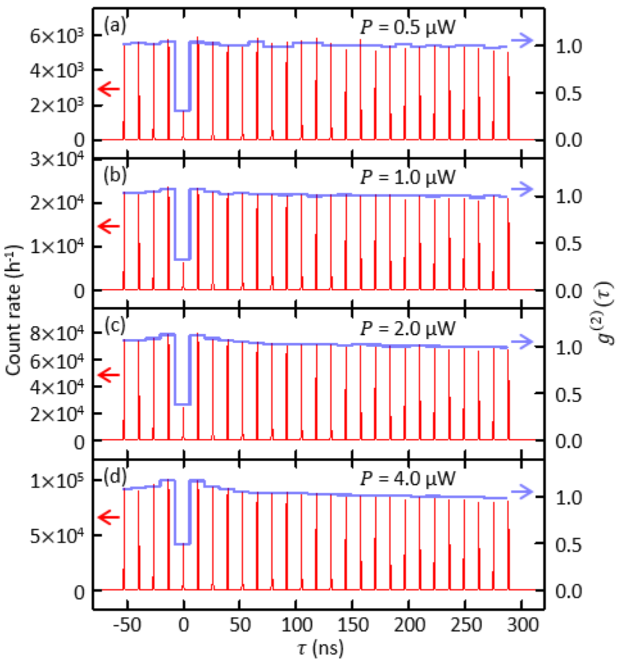


FIG. S3 Autocorrelation histograms (red lines) taken at (a) $P$ = 0.5 μW, (b) $P$ = 1.0 μW, (c) $P$ = 2.0 μW, and (d) $P$ = 4.0 μW on the device shown in Figs. 3(b) and (e). Blue lines indicate calculated second-order autocorrelation $g^{(2)}(\tau)$ for each peak.

## S4. Estimation of photon collection efficiency

In order to estimate the actual photon emission rate of the devices, we calculate the photon collection efficiency in our optical system. The objective lens has a transmittance of ~80% at the emission wavelength of around 1100 – 1200 nm, and photon collection efficiency is at most 50% as we do not expect any collection of downward emission in the suspended membrane structure of our devices. The transmission losses through the dichroic filter and long-pass filter are negligible, while the tilted band-pass filter has a transmittance of ~80%, obtained by comparing PL spectra with and without the band-pass filter (Fig. 2(a)). To obtain the coupling efficiency and transmission losses of the optical fibers, we use a CW laser with a wavelength of 1000 nm reflected from a Pt-coated substrate. We measure the power in front of the collimation lens and at the fiber end which is connected to the SSPD, where the long-pass and band-pass filters have been removed. By comparing the measured powers, the total photon transmission efficiency is found to be ~18%. The quantum efficiency of the SSPD is ~45% for the emission wavelength around 1100 – 1200 nm, and we finally obtain the total photon collection efficiency of ~2.6%.
